# Supplementary material for: Beginner's guide to visual analysis of perovskite and organic solar cell current density-voltage characteristics
Source: arXiv:2311.10553 source file (2023-11-17)

**a.**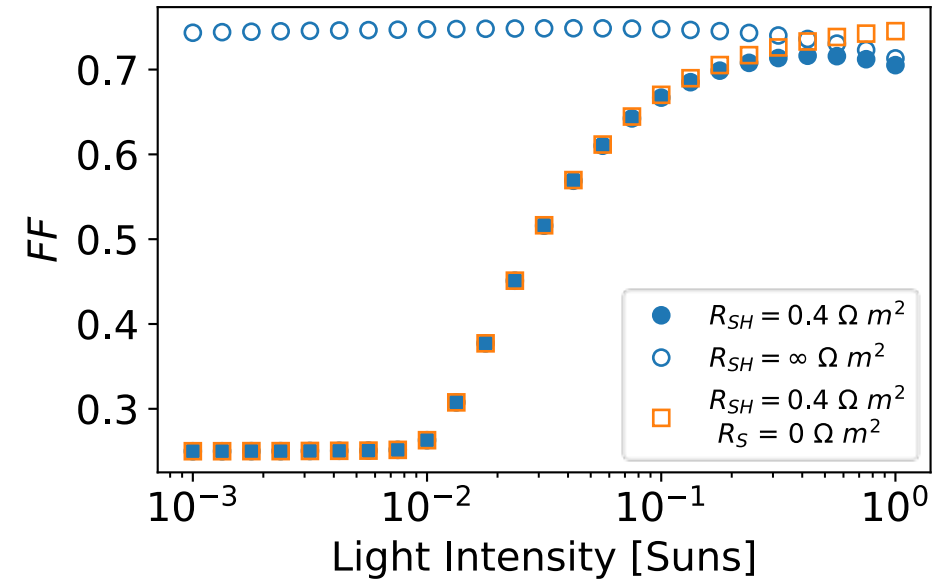**b.**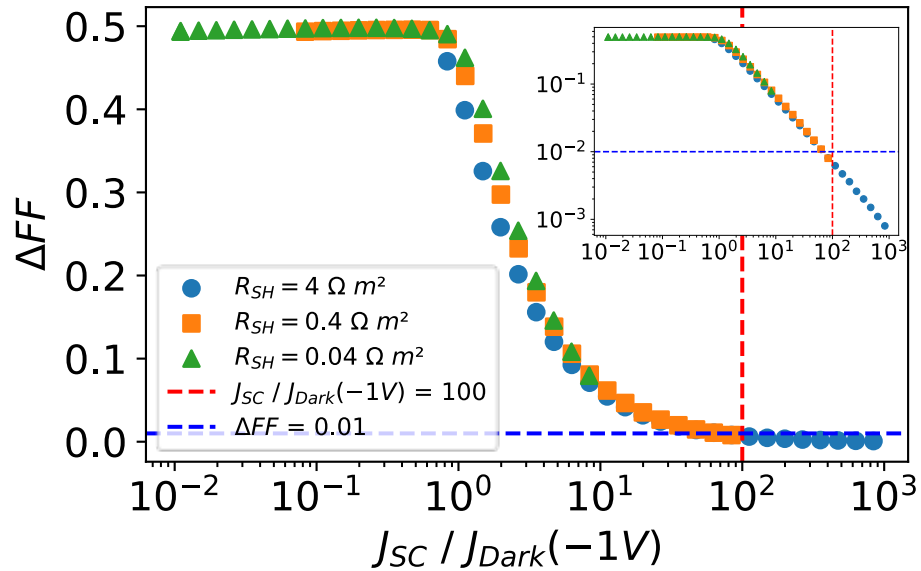

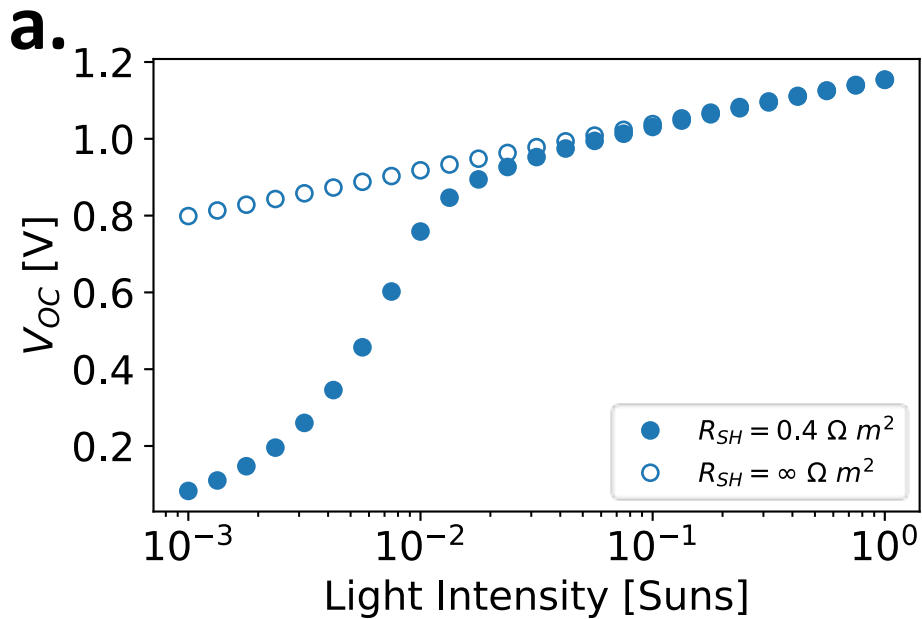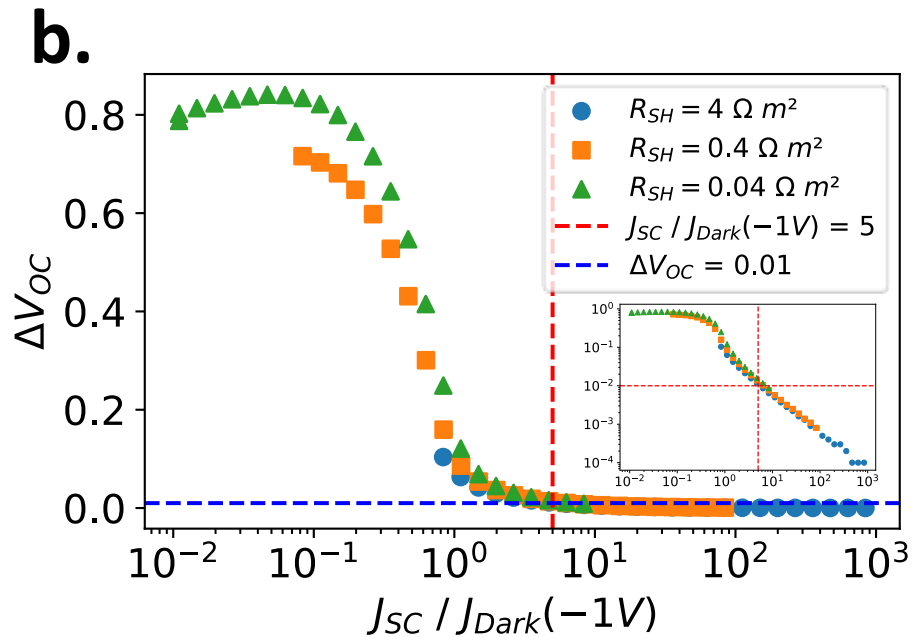

Supplement: Supplementary file 3 [file SI_fig_res_ff.pdf]
